# Supplementary material for: A Static Pruning Study on Sparse Neural Retrievers
Source: arXiv:2304.12702 source file (2023-04-25)
Supplement: Supplementary file 1 [file figure.tex]

\begin{figure}[ht]
     \centering
     \begin{subfigure}[t]{0.7\columnwidth}

         \centering
\adjustbox{max width=\textwidth}{%
         \input{appendix_tikz/compare_msmarco_index/mrr/pisa.tex}
         }
     \end{subfigure}
     \begin{subfigure}[t]{0.29\columnwidth}
         \centering
\adjustbox{max width=\textwidth}{%
         \raisebox{50px}{%
         \input{appendix_tikz/compare_msmarco_index/mrr/legend.tex}}
}
     \end{subfigure}
      \caption{Speedup vs Relative MRR@10 comparison.}
     \label{fig:rq2}
\end{figure}
