# Supplementary material for: A Static Pruning Study on Sparse Neural Retrievers
Source: arXiv:2304.12702 source file (2023-04-25)
Supplement: Supplementary file 2 [file legend.tex]

\begin{tikzpicture}
\begin{customlegend}[
legend entries={
\textsc{Eff-V-L-SPLADE~\cite{} (TC-quant)},
\textsc{Eff-V-L-SPLADE~\cite{} (DC-max)},
\textsc{DeepImpact~\cite{10.1145/3404835.3463030} (DC-max)},
\textsc{uniCOIL-Tilde~\cite{zhuang2021fast} (DC-max)},
\textsc{Eff-V-L-SPLADE~\cite{} (LS)},
\textsc{DeepImpact~\cite{10.1145/3404835.3463030} (LS)},
\textsc{uniCOIL-Tilde~\cite{zhuang2021fast} (LS)},
                        }]
         \addlegendimage{largespladeTplot};
         \addlegendimage{largespladeDplot};
         \addlegendimage{deepimpacDplot};
         \addlegendimage{unicoilDplot};
         \addlegendimage{largespladeVplot};
         \addlegendimage{deepimpacVplot};
         \addlegendimage{unicoilVplot};
        \end{customlegend}
\end{tikzpicture}
