# Supplementary material for: A Static Pruning Study on Sparse Neural Retrievers
Source: arXiv:2304.12702 source file (2023-04-25)
Supplement: Supplementary file 5 [file legend2.tex]

\begin{tikzpicture}
\begin{customlegend}[
legend columns=3,
legend entries={
\textsc{Eff-V-L-SPLADE (T)},
\textsc{Eff-V-L-SPLADE (D)},
\textsc{Eff-V-L-SPLADE (A)},
\textsc{DeepImpact (T)},
\textsc{DeepImpact (D)},
\textsc{DeepImpact (A)},
\textsc{uniCOIL-Tilde (T)},
\textsc{uniCOIL-Tilde (D)},
\textsc{uniCOIL-Tilde (A)},
\textsc{BM25 (T)},
\textsc{BM25 (D)},
\textsc{BM25 (A)}
}]
         \addlegendimage{largespladeTplot};
         \addlegendimage{largespladeDplot};
         \addlegendimage{largespladeVplot};
         \addlegendimage{deepimpacTplot};
         \addlegendimage{deepimpacDplot};
         \addlegendimage{deepimpacVplot};
         \addlegendimage{unicoilTplot};
         \addlegendimage{unicoilDplot};
         \addlegendimage{unicoilVplot};
         \addlegendimage{bmvTplot};
         \addlegendimage{bmvDplot};
         \addlegendimage{bmvVplot};
        \end{customlegend}
\end{tikzpicture}
