# Supplementary material for: A Static Pruning Study on Sparse Neural Retrievers
Source: arXiv:2304.12702 source file (2023-04-25)
Supplement: Supplementary file 6 [file figures.tex]

% \onlyinsub{
\makeatletter
\@namedef{ver@everyshi.sty}{}
\makeatother
% }

\usepackage{pgfplots, pgfplotstable}
\pgfplotsset{compat=newest}
\usepgfplotslibrary{fillbetween}

% colors for plots
\newcommand{\spladelargec}{Blue}
\newcommand{\splademediumc}{PineGreen}
\newcommand{\spladesmallc}{RubineRed}
\newcommand{\deepimpacc}{Salmon}
\newcommand{\unicoilc}{Gray}
\newcommand{\bmvc}{Black}

\pgfmathsetmacro{\stdgrad}{30}

\tikzset{every mark/.append style={solid}}
\pgfplotsset{
	grid=both, width=\linewidth, try min ticks=5,
	legend cell align=left, legend style={fill opacity=0.8},
	ylabel near ticks,
    xlabel near ticks,
    every tick label/.append style={font=\footnotesize},
}

\pgfplotsset{
    largespladeTplot/.style={thick, color=\spladelargec, mark=triangle*, mark size=2pt},
    deepimpacTplot/.style={thick, color=\deepimpacc, mark=triangle*, mark size=2pt},
    unicoilTplot/.style={thick, color=\unicoilc, mark=triangle*, mark size=2pt},
    bmvTplot/.style={thick, color=\bmvc, mark=triangle*, mark size=2pt},
    largespladeDplot/.style={thick, color=\spladelargec, mark=o, mark size=2pt},
    mediumspladeDplot/.style={thick, color=\splademediumc, mark=o, mark size=2pt},
    smallspladeDplot/.style={thick, color=\spladesmallc, mark=o, mark size=2pt},
    deepimpacDplot/.style={thick, color=\deepimpacc, mark=o, mark size=2pt}, 
    bmvDplot/.style={thick, color=\bmvc, mark=o, mark size=2pt},
    unicoilDplot/.style={thick, color=\unicoilc, mark=o, mark size=2pt},
    largespladeVplot/.style={thick, color=\spladelargec, mark=x, mark size=2pt},
    mediumspladeVplot/.style={thick, color=\splademediumc, mark=x, mark size=2pt},
    smallspladeVplot/.style={thick, color=\spladesmallc, mark=x, mark size=2pt},
    deepimpacVplot/.style={thick, color=\deepimpacc, mark=x, mark size=2pt}, 
    unicoilVplot/.style={thick, color=\unicoilc, mark=x, mark size=2pt},
    bmvVplot/.style={thick, color=\bmvc, mark=x, mark size=2pt},
    }
